# Supplementary material for: Collapse of Coherent Large Scale Flow in Strongly Turbulent Liquid Metal Convection
Source: arXiv:2110.15807 source file (2022-01-21)
Supplement: Supplementary file 1 [file SupplementaryMat_LG19130.pdf]

# Supplementary information:
# Collapse of Coherent Large Scale Flow in Strongly Turbulent Liquid Metal Convection

Felix Schindler,[1] Sven Eckert,[1] Till Zürner,[2,3] Jörg Schumacher,[2] and Tobias Vogt[1]

[1] *Helmholtz-Zentrum Dresden-Rossendorf, 01328 Dresden, Germany*

[2] *Technische Universität Ilmenau, 98684 Ilmenau, Germany*

[3] *UME, ENSTA Paris, Institut Polytechnique de Paris, 91120 Palaiseau, France*

(Dated: October 28, 2021)

## EXPERIMENTAL SETUP

The specific sensor arrangement for the cell at $\Gamma = 1$ has been described in detail in Zürner et al., J. Fluid Mech. **876**, 1108 (2019). It comprises combined temperature and velocity measurements enabling the reconstruction of the LSC structure. The same approach was followed for the new cell at $\Gamma = 0.5$, but with a significantly enhanced number of active sensors at different positions. Here, we use a total of 68 thermocouples in the convection cell and the cooling water circuits. The temperatures in both copper plates, $T_{Bot}$ and $T_{Top}$, are averaged from 8 thermocouples inside each copper block, spaced equally at a radius of $r = 140$ mm at a vertical distance of 4.5 mm from the liquid metal-copper interface. For the precise calculation of the Rayleigh number $Ra$, the temperature drop in the copper plates is evaluated by four thermocouples installed directly at the surface of the top plate, evenly distributed at a radius of $r = 114$ mm. In addition, 16 thermocouples are installed at the inner surface of the cylinder sidewall and at each of three different heights ($H/4$, $H/2$ and $3H/4$). Again, they are distributed around the circumference of the cylindrical cell. The thermocouples are calibrated to an accuracy better than 0.1 K.

High-precision PT100 temperature sensors with an accuracy of 0.001 K are used to determine the temperature change $\Delta T_w = |T_{in} - T_{out}|$ of the cooling water that is pumped through the cooling plate. Both, heating and cooling plate are temperature controlled by high-power thermostats with a temperature variation of less than 0.1 K. The Nusselt number $Nu$ is then measured by means of the volumetric flow rate $\dot{V}$ of the cooling water,

$$Nu = \frac{\dot{Q}}{\dot{Q}_{diff}} = \frac{c_{s,w}(T_w)\Delta T_w \rho_w(T_w)\dot{V}}{A\Delta T \lambda(T_m)/H}\,, \tag{1}$$

with the total heat flux absorbed by the water $\dot{Q}$, calculated with the specific heat capacity $c_{s,w}(T_w)$ and density $\rho_w(T_w)$ of the water depending on the average water temperature $T_w = (T_{in} + T_{out})/2$ in the plate. $\dot{Q}_{diff}$ is determined by means of the plate surface $A$ and the thermal conductivity of the working fluid GaInSn $\lambda(T_m)$ at the bulk temperature $T_m = (T_{Bot} + T_{Top})/2$. The Nusselt numbers are calculated at the cooling plate. The measured standard deviation of $Nu$ in shown in figure 1. To test the $Nu$-measurement accuracy, a stable temperature stratification with $\Delta T = -40$K was set up by heating the top and cooling the bottom. The resulting Nusselt number is $Nu = 0.95 \pm 0.07$. This proves that the $Nu$ measurement method is accurate and heat losses remain small. A rise of the mean temperature $T_m$ with increasing $Ra$ due to technical limitations of the cooling temperature causes a corresponding decrease in $Pr = 0.033$ at $Ra \lesssim 3 \times 10^8$ to $Pr = 0.025$ at the highest value, $Ra = 5 \times 10^9$. This point is also incorporated in the analysis as described in the main article.

## THERMAL LOSSES

The largest thermal losses occur at the largest Rayleigh numbers where the mean fluid temperature is above the ambient temperature in the laboratory. For $Ra = 5 \times 10^9$, the mean fluid temperature is by 33.5 K above the ambient laboratory temperature. The thermal conductivity of GaInSn at this temperature is 26 W/mK, that of the 20 mm thick sidewall is by a factor of 100 lower (0.25 W/mK). The conductivity of the additional 25 mm thick insulation is by a factor of about 1,000 lower (0.03 W/mK). The largest radial losses through the sidewall occur at the highest $Ra$ and are about 24 W, whereas the convective heat flux through the liquid metal is 3,300 W. At low $Ra$, the losses are correspondingly lower since we can operate the experiment closer to room temperature. The heat conduction in the side wall in the vertical direction, i.e. between the bottom and the top, results in a heat flux of 0.2 W at the highest $Ra$. In total, the thermal losses amount to about 0.7 % of the total heat flux through the liquid metal.

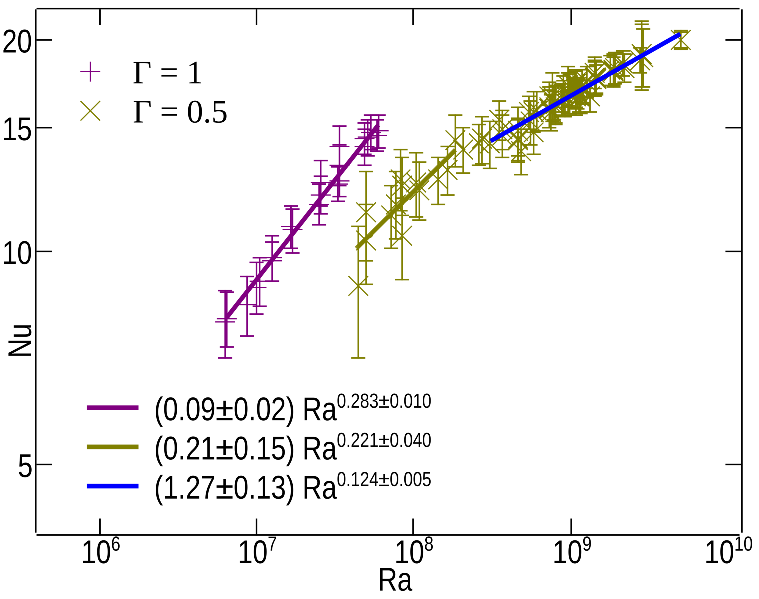


FIG. 1: Nusselt number $Nu$ and standard deviation (error bars) versus $Ra$ for aspect ratio $\Gamma = 1$ and $\Gamma = 0.5$

## SUPPLEMENTARY MOVIE

The movie shows the time evolution of the large-scale flow which is reconstructed from the UDV beamlines for the measurement at $Ra = 5 \times 10^9$, $\Gamma = 0.5$ and $Pr = 0.025$.

## EXPERIMENTAL DATA RECORD

On the following pages, we provide in Tables I to IV the data of all measurements that are presented in this publication. The reason for missing Nusselt numbers at low $Ra$ lies in the limits of measurement accuracy. For the lowest Rayleigh numbers the temperature difference between top and bottom is only 0.25 K. The temperature increase in the cooling water for tempering the top plate is again one order of magnitude lower, so that this can no longer be determined with sufficient accuracy even with the existing measurement accuracy of 0.001 K. The velocities at the lowest Rayleigh numbers can still be measured very well since the UDV system can resolve velocities as small as about 0.5 mm/s.

| $Ra$ | $\sigma(Ra)$ | $Pr$ | $Re$ | $\sigma(Re)$ | $Nu$ | $\sigma(Nu)$ | $T_{Bot}$ | $\sigma(T_{Bot})$ | $T_{Top}$ | $\sigma(T_{Top})$ | $\Delta T$ [K] |
|---|---|---|---|---|---|---|---|---|---|---|---|
| 2.32E+7 | 5.28E+5 | 0.032 | 3.99E+3 | 1.83E+3 | – | – | 24.75 | 0.01 | 24.50 | 0.01 | 0.25 |
| 2.47E+7 | 1.15E+6 | 0.032 | 4.36E+3 | 1.83E+3 | – | – | 24.74 | 0.01 | 24.48 | 0.01 | 0.27 |
| 2.91E+7 | 1.56E+6 | 0.033 | 5.23E+3 | 2.37E+3 | – | – | 20.65 | 0.01 | 20.34 | 0.02 | 0.32 |
| 3.71E+7 | 6.93E+5 | 0.033 | 6.17E+3 | 2.43E+3 | – | – | 21.28 | 0.01 | 20.87 | 0.01 | 0.41 |
| 4.31E+7 | 1.24E+6 | 0.033 | 6.48E+3 | 2.84E+3 | – | – | 21.96 | 0.01 | 21.49 | 0.01 | 0.47 |
| 4.43E+7 | 6.96E+5 | 0.032 | – | – | 8.97 | 1.89 | 22.73 | 0.01 | 22.25 | 0.01 | 0.48 |
| 4.92E+7 | 1.08E+6 | 0.033 | 6.99E+3 | 3.10E+3 | 10.40 | 1.35 | 21.13 | 0.01 | 20.59 | 0.01 | 0.54 |
| 4.93E+7 | 6.43E+5 | 0.033 | 6.57E+3 | 2.96E+3 | 11.40 | 1.65 | 21.44 | 0.01 | 20.90 | 0.01 | 0.54 |
| 5.72E+7 | 7.41E+5 | 0.029 | 6.76E+3 | 2.78E+3 | – | – | 35.17 | 0.01 | 34.56 | 0.01 | 0.61 |
| 6.22E+7 | 1.62E+6 | 0.032 | 9.03E+3 | 3.86E+3 | – | – | 23.72 | 0.02 | 23.04 | 0.01 | 0.68 |
| 7.21E+7 | 1.09E+6 | 0.033 | 8.73E+3 | 3.40E+3 | 11.30 | 1.12 | 21.22 | 0.01 | 20.43 | 0.01 | 0.79 |
| 7.73E+7 | 9.79E+5 | 0.033 | 8.27E+3 | 3.57E+3 | 11.70 | 1.28 | 21.66 | 0.01 | 20.81 | 0.01 | 0.85 |
| 8.32E+7 | 1.29E+6 | 0.033 | 9.35E+3 | 4.04E+3 | 12.70 | 1.25 | 21.33 | 0.01 | 20.42 | 0.01 | 0.91 |
| 8.34E+7 | 1.69E+6 | 0.032 | – | – | 10.60 | 1.39 | 22.92 | 0.01 | 22.00 | 0.01 | 0.91 |
| 8.37E+7 | 2.78E+6 | 0.031 | 9.35E+3 | 3.84E+3 | – | – | 26.82 | 0.03 | 25.92 | 0.05 | 0.91 |
| 8.43E+7 | 1.14E+6 | 0.033 | 9.53E+3 | 3.92E+3 | 12.40 | 1.16 | 21.64 | 0.01 | 20.72 | 0.01 | 0.92 |
| 8.44E+7 | 1.12E+6 | 0.031 | 1.01E+4 | 4.03E+3 | – | – | 27.90 | 0.03 | 26.98 | 0.03 | 0.91 |
| 8.72E+7 | 1.30E+6 | 0.031 | 1.00E+4 | 3.97E+3 | – | – | 27.73 | 0.02 | 26.78 | 0.01 | 0.94 |
| 8.87E+7 | 8.84E+5 | 0.031 | 9.37E+3 | 3.81E+3 | – | – | 26.90 | 0.01 | 25.94 | 0.01 | 0.96 |
| 9.41E+7 | 1.29E+6 | 0.031 | 9.64E+3 | 3.93E+3 | – | – | 28.49 | 0.01 | 27.48 | 0.01 | 1.02 |
| 1.02E+8 | 1.44E+6 | 0.029 | 1.09E+4 | 4.25E+3 | – | – | 35.48 | 0.01 | 34.39 | 0.01 | 1.09 |
| 1.02E+8 | 1.41E+6 | 0.032 | – | – | 12.50 | 1.29 | 23.05 | 0.01 | 21.93 | 0.01 | 1.12 |
| 1.04E+8 | 1.46E+6 | 0.031 | 1.01E+4 | 4.29E+3 | – | – | 27.04 | 0.02 | 25.91 | 0.01 | 1.13 |
| 1.09E+8 | 1.62E+6 | 0.032 | – | – | 12.20 | 1.15 | 23.14 | 0.01 | 21.95 | 0.01 | 1.19 |
| 1.11E+8 | 8.00E+5 | 0.031 | 1.07E+4 | 4.46E+3 | – | – | 28.65 | 0.01 | 27.45 | 0.01 | 1.19 |
| 1.12E+8 | 1.41E+6 | 0.031 | 1.06E+4 | 4.69E+3 | – | – | 28.62 | 0.01 | 27.41 | 0.01 | 1.21 |
| 1.22E+8 | 1.42E+6 | 0.029 | 1.13E+4 | 4.68E+3 | – | – | 35.63 | 0.01 | 34.33 | 0.01 | 1.29 |
| 1.43E+8 | 2.33E+6 | 0.032 | – | – | 12.70 | 0.98 | 23.24 | 0.01 | 21.68 | 0.02 | 1.56 |
| 1.52E+8 | 1.85E+6 | 0.031 | 1.28E+4 | 5.49E+3 | – | – | 28.84 | 0.01 | 27.20 | 0.02 | 1.64 |
| 1.61E+8 | 1.92E+6 | 0.031 | 1.24E+4 | 4.83E+3 | – | – | 27.81 | 0.02 | 26.06 | 0.02 | 1.75 |
| 1.64E+8 | 2.97E+6 | 0.033 | 1.15E+4 | 5.16E+3 | 13.10 | 1.05 | 22.32 | 0.03 | 20.53 | 0.02 | 1.80 |
| 1.65E+8 | 2.86E+6 | 0.029 | 1.25E+4 | 5.36E+3 | – | – | 35.83 | 0.01 | 34.08 | 0.02 | 1.76 |
| 1.83E+8 | 2.56E+6 | 0.032 | – | – | 14.40 | 1.20 | 23.44 | 0.02 | 21.44 | 0.02 | 2.01 |
| 2.00E+8 | 2.61E+6 | 0.031 | 1.38E+4 | 5.49E+3 | – | – | 29.12 | 0.02 | 26.97 | 0.02 | 2.15 |
| 2.00E+8 | 2.14E+6 | 0.031 | 1.37E+4 | 6.12E+3 | – | – | 29.10 | 0.01 | 26.95 | 0.02 | 2.16 |
| 2.01E+8 | 3.55E+6 | 0.032 | 1.37E+4 | 5.60E+3 | – | – | 26.16 | 0.03 | 23.98 | 0.02 | 2.18 |
| 2.05E+8 | 2.85E+6 | 0.033 | 1.47E+4 | 6.02E+3 | 14.00 | 1.02 | 22.54 | 0.02 | 20.29 | 0.02 | 2.25 |
| 2.12E+8 | 2.93E+6 | 0.029 | 1.43E+4 | 6.16E+3 | – | – | 36.11 | 0.02 | 33.86 | 0.02 | 2.25 |
| 2.45E+8 | 2.39E+6 | 0.031 | 1.41E+4 | 6.34E+3 | – | – | 29.34 | 0.01 | 26.69 | 0.02 | 2.65 |
| 2.58E+8 | 2.96E+6 | 0.033 | 1.59E+4 | 6.21E+3 | 14.20 | 0.93 | 22.87 | 0.02 | 20.05 | 0.02 | 2.82 |
| 2.71E+8 | 3.75E+6 | 0.032 | – | – | 14.40 | 1.08 | 23.97 | 0.02 | 21.01 | 0.03 | 2.97 |
| 2.98E+8 | 3.81E+6 | 0.031 | 1.64E+4 | 7.25E+3 | – | – | 28.32 | 0.03 | 25.10 | 0.03 | 3.22 |
| 3.03E+8 | 4.18E+6 | 0.033 | 1.59E+4 | 6.86E+3 | 14.20 | 1.08 | 23.32 | 0.02 | 20.01 | 0.03 | 3.31 |
| 3.07E+8 | 3.80E+6 | 0.029 | 1.67E+4 | 7.15E+3 | – | – | 36.60 | 0.02 | 33.34 | 0.03 | 3.26 |
| 3.50E+8 | 4.21E+6 | 0.032 | – | – | 15.40 | 0.98 | 26.30 | 0.02 | 22.50 | 0.03 | 3.81 |
| 3.62E+8 | 4.49E+6 | 0.032 | 1.81E+4 | 7.39E+3 | 14.60 | 1.01 | 24.50 | 0.03 | 20.60 | 0.03 | 3.96 |
| 3.62E+8 | 4.61E+6 | 0.032 | 1.79E+4 | 7.47E+3 | 14.90 | 0.94 | 24.50 | 0.03 | 20.60 | 0.03 | 3.96 |
| 3.73E+8 | 4.09E+6 | 0.031 | 1.87E+4 | 7.76E+3 | – | – | 30.10 | 0.02 | 26.00 | 0.03 | 4.03 |
| 3.75E+8 | 4.03E+6 | 0.031 | 1.76E+4 | 7.70E+3 | – | – | 30.10 | 0.02 | 26.00 | 0.03 | 4.05 |
| 3.80E+8 | 6.21E+6 | 0.031 | 1.84E+4 | 7.51E+3 | – | – | 30.10 | 0.03 | 26.00 | 0.04 | 4.11 |
| 3.91E+8 | 4.90E+6 | 0.029 | 1.85E+4 | 8.25E+3 | – | – | 37.10 | 0.03 | 33.00 | 0.04 | 4.16 |
| 4.59E+8 | 6.16E+6 | 0.031 | 1.99E+4 | 7.75E+3 | 14.40 | 1.00 | 30.50 | 0.04 | 25.60 | 0.03 | 4.96 |
| 4.60E+8 | 5.99E+6 | 0.031 | 1.96E+4 | 8.33E+3 | 14.50 | 1.01 | 30.60 | 0.04 | 25.60 | 0.04 | 4.96 |
| 4.64E+8 | 5.89E+6 | 0.031 | 1.99E+4 | 8.52E+3 | 14.90 | 1.17 | 30.60 | 0.03 | 25.60 | 0.04 | 5.01 |
| 4.80E+8 | 5.54E+6 | 0.029 | 2.00E+4 | 8.45E+3 | 13.90 | 1.01 | 37.60 | 0.03 | 32.40 | 0.04 | 5.11 |

TABLE I: Data table for the conducted laboratory experiments at aspect ratio $\Gamma = 0.5$. First and second columns show the Rayleigh number $Ra$ and the corresponding standard deviation $\sigma(Ra)$, the next column shows the Prandtl number $Pr$, the fourth and fifth columns show the Reynolds numbers $Re$ and the corresponding standard deviation $\sigma(Re)$. The sixth and seventh columns show the Nusselt number $Nu$ and the corresponding standard deviation $\sigma(Nu)$. Columns eight through eleven show the temperatures and standard deviations for the bottom and top temperatures in units of Celsius. The last column shows the temperature difference between the bottom and the top in Kelvin. Table entries with – are due to measuring range limits or sensor failures and were excluded from the analysis in the main text.

| $Ra$ | $\sigma(Ra)$ | $Pr$ | $Re$ | $\sigma(Re)$ | $Nu$ | $\sigma(Nu)$ | $T_{Bot}$ | $\sigma(T_{Bot})$ | $T_{Top}$ | $\sigma(T_{Top})$ | $\Delta T$ [K] |
|---|---|---|---|---|---|---|---|---|---|---|---|
| 5.43E+8 | 6.19E+6 | 0.032 | – | – | 15.80 | 0.84 | 28.50 | 0.04 | 22.60 | 0.04 | 5.90 |
| 5.50E+8 | 6.60E+6 | 0.031 | 2.20E+4 | 9.24E+3 | 15.30 | 1.10 | 31.00 | 0.04 | 25.10 | 0.04 | 5.93 |
| 5.73E+8 | 6.21E+6 | 0.029 | 2.26E+4 | 8.81E+3 | 14.70 | 0.96 | 38.10 | 0.04 | 32.00 | 0.04 | 6.10 |
| 5.82E+8 | 6.57E+6 | 0.031 | 2.15E+4 | 9.32E+3 | 15.80 | 1.07 | 32.30 | 0.04 | 26.10 | 0.04 | 6.27 |
| 6.11E+8 | 7.21E+6 | 0.032 | 2.25E+4 | 8.98E+3 | 15.90 | 0.99 | 28.80 | 0.04 | 22.20 | 0.05 | 6.63 |
| 7.21E+8 | 8.65E+6 | 0.031 | 2.28E+4 | 1.04E+4 | 16.10 | 1.09 | 31.90 | 0.05 | 24.20 | 0.05 | 7.78 |
| 7.22E+8 | 7.88E+6 | 0.031 | – | – | 16.60 | 0.78 | 30.40 | 0.04 | 22.60 | 0.05 | 7.82 |
| 7.22E+8 | 8.89E+6 | 0.031 | 2.44E+4 | 1.01E+4 | 16.00 | 0.96 | 32.00 | 0.05 | 24.20 | 0.05 | 7.79 |
| 7.45E+8 | 8.78E+6 | 0.029 | 2.55E+4 | 1.08E+4 | 15.80 | 0.91 | 39.00 | 0.05 | 31.10 | 0.05 | 7.93 |
| 7.60E+8 | 7.95E+6 | 0.031 | 2.38E+4 | 1.02E+4 | 16.60 | 1.29 | 33.40 | 0.05 | 25.20 | 0.06 | 8.19 |
| 7.85E+8 | 8.85E+6 | 0.031 | 2.35E+4 | 1.00E+4 | 16.20 | 0.87 | 30.80 | 0.05 | 22.30 | 0.05 | 8.50 |
| 7.96E+8 | 9.26E+6 | 0.031 | 2.50E+4 | 1.03E+4 | 16.20 | 0.97 | 32.80 | 0.05 | 24.20 | 0.06 | 8.58 |
| 8.03E+8 | 7.82E+6 | 0.030 | 2.51E+4 | 9.88E+3 | 16.00 | 0.85 | 34.90 | 0.05 | 26.30 | 0.06 | 8.62 |
| 8.82E+8 | 9.68E+6 | 0.031 | 2.53E+4 | 1.09E+4 | 16.50 | 0.83 | 32.80 | 0.06 | 23.20 | 0.05 | 9.52 |
| 8.92E+8 | 9.99E+6 | 0.031 | 2.61E+4 | 1.06E+4 | 16.80 | 1.00 | 32.80 | 0.05 | 23.20 | 0.06 | 9.63 |
| 8.95E+8 | 9.09E+6 | 0.031 | – | – | 16.80 | 0.71 | 32.30 | 0.05 | 22.70 | 0.06 | 9.67 |
| 9.27E+8 | 1.05E+7 | 0.029 | 2.70E+4 | 1.12E+4 | 16.40 | 0.87 | 40.00 | 0.07 | 30.10 | 0.06 | 9.87 |
| 9.59E+8 | 1.07E+7 | 0.029 | 2.66E+4 | 1.11E+4 | 16.80 | 1.12 | 39.40 | 0.06 | 29.20 | 0.07 | 10.20 |
| 9.62E+8 | 1.09E+7 | 0.029 | 2.83E+4 | 1.15E+4 | 17.20 | 1.13 | 40.50 | 0.06 | 30.20 | 0.07 | 10.20 |
| 9.84E+8 | 9.90E+6 | 0.030 | 2.71E+4 | 1.16E+4 | 16.80 | 1.05 | 38.80 | 0.05 | 28.30 | 0.07 | 10.50 |
| 1.06E+9 | 1.18E+7 | 0.031 | – | – | 17.30 | 0.76 | 34.30 | 0.07 | 22.80 | 0.07 | 11.50 |
| 1.07E+9 | 1.17E+7 | 0.031 | 2.81E+4 | 1.21E+4 | 17.30 | 0.76 | 34.30 | 0.07 | 22.80 | 0.07 | 11.50 |
| 1.07E+9 | 1.18E+7 | 0.031 | – | – | 17.30 | 0.75 | 34.30 | 0.07 | 22.80 | 0.07 | 11.50 |
| 1.07E+9 | 1.22E+7 | 0.031 | 2.82E+4 | 1.12E+4 | 16.60 | 0.99 | 34.80 | 0.07 | 23.30 | 0.07 | 11.50 |
| 1.07E+9 | 1.15E+7 | 0.031 | – | – | 17.40 | 0.79 | 34.40 | 0.07 | 22.80 | 0.07 | 11.60 |
| 1.08E+9 | 1.17E+7 | 0.031 | – | – | 17.10 | 0.87 | 33.70 | 0.07 | 22.10 | 0.07 | 11.60 |
| 1.08E+9 | 1.13E+7 | 0.031 | 2.75E+4 | 1.20E+4 | 17.00 | 1.02 | 34.00 | 0.06 | 22.40 | 0.07 | 11.60 |
| 1.10E+9 | 1.20E+7 | 0.029 | 2.83E+4 | 1.22E+4 | 16.80 | 0.87 | 40.80 | 0.07 | 29.20 | 0.07 | 11.60 |
| 1.13E+9 | 1.17E+7 | 0.027 | – | – | 16.60 | 0.88 | 50.90 | 0.07 | 39.10 | 0.07 | 11.80 |
| 1.15E+9 | 1.26E+7 | 0.031 | 2.84E+4 | 1.16E+4 | 16.60 | 0.92 | 35.30 | 0.08 | 22.80 | 0.07 | 12.40 |
| 1.18E+9 | 1.29E+7 | 0.029 | 3.07E+4 | 1.26E+4 | 17.20 | 0.91 | 41.30 | 0.08 | 28.80 | 0.07 | 12.60 |
| 1.18E+9 | 1.22E+7 | 0.030 | 2.85E+4 | 1.22E+4 | 17.20 | 0.98 | 36.40 | 0.07 | 23.70 | 0.07 | 12.70 |
| 1.27E+9 | 1.41E+7 | 0.029 | – | – | 17.40 | 0.89 | 41.80 | 0.09 | 28.30 | 0.08 | 13.50 |
| 1.32E+9 | 1.32E+7 | 0.027 | – | – | 16.60 | 0.82 | 51.90 | 0.08 | 38.10 | 0.07 | 13.80 |
| 1.41E+9 | 1.51E+7 | 0.030 | 3.13E+4 | 1.31E+4 | 17.70 | 0.98 | 40.50 | 0.08 | 25.50 | 0.09 | 15.00 |
| 1.41E+9 | 1.48E+7 | 0.030 | 3.09E+4 | 1.37E+4 | 17.90 | 0.89 | 40.50 | 0.08 | 25.40 | 0.09 | 15.10 |
| 1.41E+9 | 1.61E+7 | 0.030 | 3.15E+4 | 1.42E+4 | 17.60 | 0.99 | 40.60 | 0.09 | 25.50 | 0.10 | 15.10 |
| 1.44E+9 | 1.44E+7 | 0.029 | 3.37E+4 | 1.35E+4 | 17.70 | 0.94 | 45.60 | 0.08 | 30.40 | 0.09 | 15.20 |
| 1.44E+9 | 1.65E+7 | 0.029 | – | – | 17.60 | 0.88 | 42.70 | 0.10 | 27.40 | 0.09 | 15.30 |
| 1.78E+9 | 1.94E+7 | 0.029 | – | – | 18.10 | 0.88 | 44.50 | 0.11 | 25.60 | 0.11 | 18.90 |
| 1.86E+9 | 1.85E+7 | 0.028 | 3.26E+4 | 1.30E+4 | 18.00 | 0.90 | 52.00 | 0.10 | 32.50 | 0.12 | 19.50 |
| 1.88E+9 | 1.88E+7 | 0.028 | 3.61E+4 | 1.54E+4 | 18.10 | 0.92 | 49.40 | 0.11 | 29.60 | 0.11 | 19.80 |
| 1.90E+9 | 1.83E+7 | 0.029 | 3.67E+4 | 1.53E+4 | 18.20 | 0.92 | 45.90 | 0.10 | 25.60 | 0.11 | 20.20 |
| 2.13E+9 | 2.16E+7 | 0.029 | – | – | 18.50 | 0.78 | 46.30 | 0.12 | 23.70 | 0.12 | 22.60 |
| 2.22E+9 | 2.19E+7 | 0.027 | – | – | 18.20 | 0.81 | 56.70 | 0.12 | 33.60 | 0.12 | 23.10 |
| 2.73E+9 | 2.49E+7 | 0.027 | – | – | 18.70 | 0.77 | 60.60 | 0.15 | 32.20 | 0.13 | 28.50 |
| 2.81E+9 | 2.60E+7 | 0.028 | 4.09E+4 | 1.70E+4 | 19.10 | 2.13 | 55.60 | 0.14 | 26.00 | 0.15 | 29.60 |
| 2.82E+9 | 2.54E+7 | 0.028 | 4.30E+4 | 1.79E+4 | 19.10 | 1.90 | 55.60 | 0.14 | 26.00 | 0.15 | 29.60 |
| 2.86E+9 | 2.65E+7 | 0.028 | 4.20E+4 | 1.81E+4 | 18.90 | 1.79 | 56.10 | 0.15 | 26.00 | 0.16 | 30.10 |
| 4.99E+9 | 3.85E+7 | 0.025 | 5.57E+4 | 2.38E+4 | 20.00 | 0.54 | 80.10 | 0.20 | 28.90 | 0.22 | 51.20 |
| 4.99E+9 | 3.91E+7 | 0.025 | 5.44E+4 | 2.37E+4 | 19.90 | 0.53 | 80.10 | 0.20 | 28.90 | 0.22 | 51.20 |

TABLE II: Continuation of Table I.

| $Ra$ | $\sigma(Ra)$ | $Pr$ | $Re$ | $\sigma(Re)$ | $Nu$ | $\sigma(Nu)$ | $T_{Bot}$ | $\sigma(T_{Bot})$ | $T_{Top}$ | $\sigma(T_{Top})$ | $\Delta T$ [K] |
|---|---|---|---|---|---|---|---|---|---|---|---|
| 4.37E+5 | 2.35E+4 | 0.029 | 2.11E+3 | 2.47E+2 | – | – | 35.11 | 0.01 | 34.90 | 0.01 | 0.21 |
| 6.12E+5 | 2.98E+4 | 0.029 | 2.44E+3 | 3.68E+2 | – | – | 35.14 | 0.01 | 34.85 | 0.01 | 0.29 |
| 6.23E+5 | 2.88E+4 | 0.029 | 2.26E+3 | 4.17E+2 | – | – | 35.15 | 0.01 | 34.85 | 0.01 | 0.30 |
| 6.78E+5 | 2.82E+4 | 0.029 | 2.68E+3 | 3.74E+2 | – | – | 35.18 | 0.01 | 34.85 | 0.01 | 0.32 |
| 9.69E+5 | 3.73E+4 | 0.029 | 2.97E+3 | 5.90E+2 | – | – | 35.21 | 0.01 | 34.75 | 0.01 | 0.46 |
| 9.89E+5 | 3.27E+4 | 0.029 | 2.80E+3 | 5.53E+2 | – | – | 35.22 | 0.01 | 34.75 | 0.01 | 0.47 |
| 1.01E+6 | 3.50E+4 | 0.029 | 2.96E+3 | 6.14E+2 | – | – | 35.24 | 0.02 | 34.75 | 0.01 | 0.49 |
| 1.04E+6 | 3.07E+4 | 0.029 | 2.77E+3 | 6.05E+2 | – | – | 35.25 | 0.01 | 34.75 | 0.01 | 0.50 |
| 1.04E+6 | 3.65E+4 | 0.029 | 2.99E+3 | 6.04E+2 | – | – | 35.25 | 0.02 | 34.75 | 0.01 | 0.50 |
| 1.06E+6 | 2.23E+4 | 0.029 | 2.78E+3 | 6.05E+2 | – | – | 35.26 | 0.01 | 34.75 | 0.01 | 0.51 |
| 1.11E+6 | 4.03E+4 | 0.029 | 3.10E+3 | 7.49E+2 | – | – | 35.28 | 0.02 | 34.75 | 0.01 | 0.53 |
| 1.11E+6 | 4.04E+4 | 0.029 | 2.98E+3 | 6.19E+2 | – | – | 35.28 | 0.02 | 34.75 | 0.01 | 0.53 |
| 1.57E+6 | 4.76E+4 | 0.029 | 3.29E+3 | 6.93E+2 | – | – | 35.38 | 0.02 | 34.63 | 0.01 | 0.75 |
| 1.60E+6 | 4.31E+4 | 0.029 | 3.33E+3 | 7.76E+2 | – | – | 35.40 | 0.02 | 34.63 | 0.01 | 0.77 |
| 1.66E+6 | 4.72E+4 | 0.029 | 3.46E+3 | 9.42E+2 | – | – | 35.42 | 0.02 | 34.63 | 0.01 | 0.79 |
| 1.66E+6 | 6.82E+4 | 0.029 | 3.56E+3 | 8.18E+2 | – | – | 35.43 | 0.03 | 34.63 | 0.02 | 0.79 |
| 1.73E+6 | 5.87E+4 | 0.029 | 3.71E+3 | 8.28E+2 | – | – | 35.44 | 0.03 | 34.61 | 0.02 | 0.83 |
| 2.01E+6 | 4.70E+4 | 0.029 | 3.61E+3 | 8.59E+2 | – | – | 35.46 | 0.02 | 34.50 | 0.01 | 0.96 |
| 2.09E+6 | 5.89E+4 | 0.029 | 3.74E+3 | 8.98E+2 | – | – | 35.50 | 0.02 | 34.50 | 0.02 | 1.00 |
| 2.09E+6 | 4.94E+4 | 0.029 | 3.82E+3 | 1.08E+3 | – | – | 35.50 | 0.02 | 34.50 | 0.02 | 1.00 |
| 2.10E+6 | 3.63E+4 | 0.029 | 4.12E+3 | 7.45E+2 | – | – | 35.51 | 0.02 | 34.50 | 0.01 | 1.01 |
| 2.11E+6 | 5.44E+4 | 0.029 | 3.49E+3 | 9.02E+2 | – | – | 35.51 | 0.03 | 34.50 | 0.01 | 1.01 |
| 2.17E+6 | 7.74E+4 | 0.029 | 4.06E+3 | 8.74E+2 | – | – | 35.54 | 0.03 | 34.50 | 0.02 | 1.04 |
| 2.18E+6 | 5.22E+4 | 0.029 | 4.23E+3 | 1.10E+3 | – | – | 35.54 | 0.02 | 34.50 | 0.02 | 1.04 |
| 2.27E+6 | 5.29E+4 | 0.029 | 3.92E+3 | 9.36E+2 | – | – | 35.59 | 0.03 | 34.50 | 0.01 | 1.09 |
| 2.30E+6 | 5.90E+4 | 0.029 | 3.94E+3 | 9.16E+2 | – | – | 35.60 | 0.03 | 34.50 | 0.01 | 1.10 |
| 3.12E+6 | 7.09E+4 | 0.029 | 4.67E+3 | 1.08E+3 | – | – | 35.74 | 0.03 | 34.25 | 0.02 | 1.49 |
| 3.13E+6 | 7.82E+4 | 0.029 | 4.21E+3 | 1.33E+3 | – | – | 35.75 | 0.03 | 34.25 | 0.03 | 1.50 |
| 3.20E+6 | 8.65E+4 | 0.029 | 4.49E+3 | 1.13E+3 | – | – | 35.78 | 0.04 | 34.25 | 0.02 | 1.53 |
| 4.15E+6 | 1.67E+5 | 0.029 | 4.73E+3 | 1.54E+3 | – | – | 35.98 | 0.05 | 34.00 | 0.06 | 1.98 |
| 4.18E+6 | 1.32E+5 | 0.029 | 5.01E+3 | 1.53E+3 | – | – | 36.00 | 0.04 | 34.00 | 0.05 | 2.00 |
| 4.18E+6 | 1.01E+5 | 0.029 | 4.99E+3 | 1.57E+3 | – | – | 36.00 | 0.04 | 34.00 | 0.03 | 2.00 |
| 4.19E+6 | 1.45E+5 | 0.029 | 5.22E+3 | 1.29E+3 | – | – | 36.00 | 0.06 | 34.00 | 0.04 | 2.00 |
| 6.28E+6 | 2.29E+5 | 0.029 | 6.02E+3 | 1.48E+3 | 7.95 | 0.89 | 36.50 | 0.05 | 33.50 | 0.08 | 3.01 |
| 6.35E+6 | 1.57E+5 | 0.029 | 6.16E+3 | 1.51E+3 | – | – | 36.54 | 0.05 | 33.50 | 0.06 | 3.03 |
| 6.46E+6 | 1.40E+5 | 0.029 | 6.04E+3 | 1.46E+3 | – | – | 36.59 | 0.06 | 33.50 | 0.03 | 3.09 |
| 6.50E+6 | 1.88E+5 | 0.029 | 6.24E+3 | 1.46E+3 | 8.06 | 0.72 | 36.61 | 0.06 | 33.50 | 0.06 | 3.11 |
| 8.39E+6 | 2.27E+5 | 0.029 | 6.74E+3 | 1.75E+3 | – | – | 37.01 | 0.10 | 33.00 | 0.04 | 4.01 |
| 8.69E+6 | 2.90E+5 | 0.029 | 6.87E+3 | 1.71E+3 | 8.43 | 0.81 | 37.15 | 0.08 | 33.00 | 0.11 | 4.15 |
| 8.79E+6 | 2.38E+5 | 0.029 | 7.02E+3 | 1.72E+3 | – | – | 37.21 | 0.08 | 33.00 | 0.07 | 4.21 |
| 8.81E+6 | 2.38E+5 | 0.029 | 7.00E+3 | 1.70E+3 | – | – | 37.21 | 0.08 | 33.00 | 0.07 | 4.21 |

TABLE III: Data table for the conducted laboratory experiments at aspect ratio $\Gamma = 1$. First and second columns show the Rayleigh number $Ra$ and the corresponding standard deviation $\sigma(Ra)$, the next column shows the Prandtl number $Pr$, the fourth and fifth columns show the Reynolds numbers $Re$ and the corresponding standard deviation $\sigma(Re)$. The sixth and seventh columns show the Nusselt number $Nu$ and the corresponding standard deviation $\sigma(Nu)$. Columns eight through eleven show the temperatures and standard deviations for the bottom and top temperatures in units of Celsius. The last column shows the temperature difference between the bottom and the top in Kelvin. Table entries with – are due to measuring range limits or sensor failures and were excluded from the analysis in the main text.

| $Ra$ | $\sigma(Ra)$ | $Pr$ | $Re$ | $\sigma(Re)$ | $Nu$ | $\sigma(Nu)$ | $T_{Bot}$ | $\sigma(T_{Bot})$ | $T_{Top}$ | $\sigma(T_{Top})$ | $\Delta T$ [K] |
|---|---|---|---|---|---|---|---|---|---|---|---|
| 9.93E+6 | 4.98E+5 | 0.029 | 7.19E+3 | 1.86E+3 | 8.94 | 0.76 | 37.25 | 0.22 | 32.50 | 0.11 | 4.75 |
| 1.01E+7 | 2.99E+5 | 0.029 | 7.57E+3 | 1.77E+3 | – | – | 37.34 | 0.11 | 32.50 | 0.09 | 4.84 |
| 1.03E+7 | 2.55E+5 | 0.029 | 7.68E+3 | 1.91E+3 | – | – | 37.43 | 0.09 | 32.50 | 0.08 | 4.94 |
| 1.05E+7 | 2.67E+5 | 0.029 | 7.45E+3 | 1.95E+3 | 9.10 | 0.71 | 37.50 | 0.08 | 32.50 | 0.09 | 5.00 |
| 1.05E+7 | 3.00E+5 | 0.029 | 7.33E+3 | 1.92E+3 | – | – | 37.51 | 0.09 | 32.50 | 0.06 | 5.01 |
| 1.05E+7 | 2.98E+5 | 0.029 | 7.51E+3 | 1.98E+3 | – | – | 37.54 | 0.11 | 32.50 | 0.09 | 5.04 |
| 1.26E+7 | 2.98E+5 | 0.029 | 7.91E+3 | 2.09E+3 | 9.81 | 0.73 | 38.00 | 0.09 | 32.00 | 0.10 | 6.00 |
| 1.26E+7 | 3.60E+5 | 0.029 | 8.23E+3 | 1.98E+3 | 9.72 | 0.61 | 38.04 | 0.10 | 32.00 | 0.10 | 6.04 |
| 1.27E+7 | 3.26E+5 | 0.029 | 8.35E+3 | 1.97E+3 | – | – | 38.06 | 0.10 | 32.00 | 0.10 | 6.06 |
| 1.67E+7 | 3.94E+5 | 0.029 | 8.74E+3 | 2.75E+3 | 10.90 | 0.75 | 38.97 | 0.13 | 31.00 | 0.12 | 7.97 |
| 1.67E+7 | 4.39E+5 | 0.029 | 9.31E+3 | 2.36E+3 | 10.80 | 0.77 | 39.00 | 0.13 | 31.00 | 0.13 | 8.00 |
| 2.51E+7 | 5.82E+5 | 0.029 | 9.87E+3 | 3.28E+3 | 11.70 | 0.76 | 40.99 | 0.19 | 29.00 | 0.17 | 11.99 |
| 2.53E+7 | 6.08E+5 | 0.029 | 1.08E+4 | 2.86E+3 | 12.10 | 0.73 | 41.11 | 0.21 | 29.00 | 0.17 | 12.11 |
| 2.54E+7 | 5.39E+5 | 0.029 | 1.07E+4 | 2.95E+3 | 12.50 | 0.90 | 41.13 | 0.21 | 29.00 | 0.15 | 12.13 |
| 2.55E+7 | 5.50E+5 | 0.029 | 1.12E+4 | 2.75E+3 | – | – | 41.18 | 0.19 | 29.00 | 0.16 | 12.18 |
| 3.22E+7 | 8.35E+5 | 0.029 | 1.19E+4 | 3.27E+3 | – | – | 42.46 | 0.24 | 27.04 | 0.26 | 15.42 |
| 3.32E+7 | 8.78E+5 | 0.029 | 1.25E+4 | 3.99E+3 | 12.50 | 0.69 | 42.90 | 0.26 | 27.03 | 0.26 | 15.87 |
| 3.34E+7 | 7.07E+5 | 0.029 | 1.17E+4 | 3.73E+3 | 12.60 | 0.63 | 43.00 | 0.17 | 27.01 | 0.24 | 15.99 |
| 3.35E+7 | 6.54E+5 | 0.029 | 1.21E+4 | 3.32E+3 | 14.10 | 0.92 | 43.00 | 0.22 | 27.00 | 0.19 | 16.00 |
| 3.39E+7 | 6.76E+5 | 0.029 | 1.25E+4 | 3.41E+3 | 13.30 | 0.86 | 43.20 | 0.26 | 27.00 | 0.19 | 16.20 |
| 4.82E+7 | 1.00E+6 | 0.029 | 1.46E+4 | 3.92E+3 | 14.50 | 0.74 | 46.78 | 0.36 | 23.72 | 0.28 | 23.06 |
| 4.85E+7 | 9.69E+5 | 0.029 | 1.44E+4 | 3.96E+3 | 14.10 | 0.84 | 47.41 | 0.36 | 24.24 | 0.29 | 23.17 |
| 5.11E+7 | 9.77E+5 | 0.029 | 1.46E+4 | 4.10E+3 | 14.50 | 0.84 | 47.94 | 0.34 | 23.53 | 0.36 | 24.41 |
| 5.28E+7 | 9.76E+5 | 0.029 | 1.51E+4 | 4.22E+3 | 14.80 | 0.81 | 47.97 | 0.35 | 22.73 | 0.31 | 25.24 |
| 5.75E+7 | 1.07E+6 | 0.029 | 1.60E+4 | 4.43E+3 | – | – | 49.02 | 0.34 | 21.52 | 0.29 | 27.50 |
| 5.81E+7 | 1.12E+6 | 0.029 | 1.54E+4 | 4.28E+3 | 14.60 | 0.74 | 49.01 | 0.40 | 21.23 | 0.34 | 27.78 |
| 5.81E+7 | 1.18E+6 | 0.028 | 1.57E+4 | 4.21E+3 | – | – | 53.32 | 0.40 | 25.76 | 0.38 | 27.56 |
| 5.88E+7 | 1.10E+6 | 0.029 | 1.54E+4 | 4.46E+3 | – | – | 49.34 | 0.32 | 21.21 | 0.37 | 28.12 |
| 5.89E+7 | 1.28E+6 | 0.028 | 1.61E+4 | 4.48E+3 | – | – | 53.57 | 0.50 | 25.65 | 0.38 | 27.92 |
| 5.93E+7 | 1.30E+6 | 0.028 | 1.52E+4 | 4.43E+3 | 14.80 | 0.80 | 54.39 | 0.44 | 26.31 | 0.39 | 28.08 |
| 6.01E+7 | 1.27E+6 | 0.029 | 1.57E+4 | 4.25E+3 | – | – | 50.18 | 0.50 | 21.48 | 0.35 | 28.71 |

TABLE IV: Continuation of Table III.
